# Supplementary material for: Relational Algebra and Calculus with SQL Null Values
Source: arXiv:2202.10898 source file (2022-02-22)
Supplement: Supplementary file 1 [file appendix.tex]

\newpage
\appendix
\section{First-order fragment of SQL \fosql and Relational Algebra with null values \nRA}\label{appendix:fosql}

%\begin{figure}[h]
%\begin{verbatim}
%create-table := CREATE TABLE table ( { column , { VARCHAR | INT } }+ ) ;
%
%query := SELECT DISTINCT { expression [ AS column ] }+ 
%         FROM { table [ AS table ] | query AS table }+ 
%         WHERE condition ;
%         | query { UNION | INTERSECT | EXCEPT } query ;
%
%condition := atomic-condition | (condition) 
%             | condition { AND | OR } condition
%             | NOT condition 
%
%atomic-condition := simple-comparison
%                    | [ NOT ] EXISTS query
%                    | { expression }+ [ NOT ] IN ({ query | { expression }+ })
%                  
%simple-comparison := expression { = | != | > | < | >= | <= } expression
%                     | expression IS [ NOT ] NULL
%
%expression := table.column | value
%
%value := string | number | NULL
%\end{verbatim}
%\caption{The syntax of \fosql}
%\label{fig:fosql}
%\end{figure}

We define  \fosql\!\!, a first-order fragment of \sql with set-based semantics, with the purpose of comparing it with relational algebra. In this appendix we show the equivalence between \fosql and \nRA. 

{\small
\begin{verbatim}
create-table := CREATE TABLE table 
                 ( { column { TEXT | INTEGER } [ NOT ] NULL , }+
                   { CONSTRAINT constraint-name CHECK (condition) , }* ;

query := SELECT DISTINCT { expression [ AS column ] }+ 
         FROM { table [ AS table ] | query AS table }+ 
         WHERE condition ;
         | query { UNION | INTERSECT | EXCEPT } query ;

condition := atomic-condition | (condition) 
             | condition { AND | OR } condition
             | NOT condition 

atomic-condition := simple-comparison
                    | [ NOT ] EXISTS query
                    | { expression }+ [ NOT ] IN 
                          ({ query | { expression }+ })
                  
simple-comparison := expression { = | != | > | < | >= | <= } expression
                     | expression IS [ NOT ] NULL

expression := table.column | value

value := string | number | NULL
\end{verbatim}
}

We first observe that in \fosql the impact of null values is only in the evaluation of the truth value of conditions in the \texttt{WHERE} clause, which should be evaluated under three-valued (true, false, and unknown) logic semantics:

\includegraphics[width=.3\textwidth]{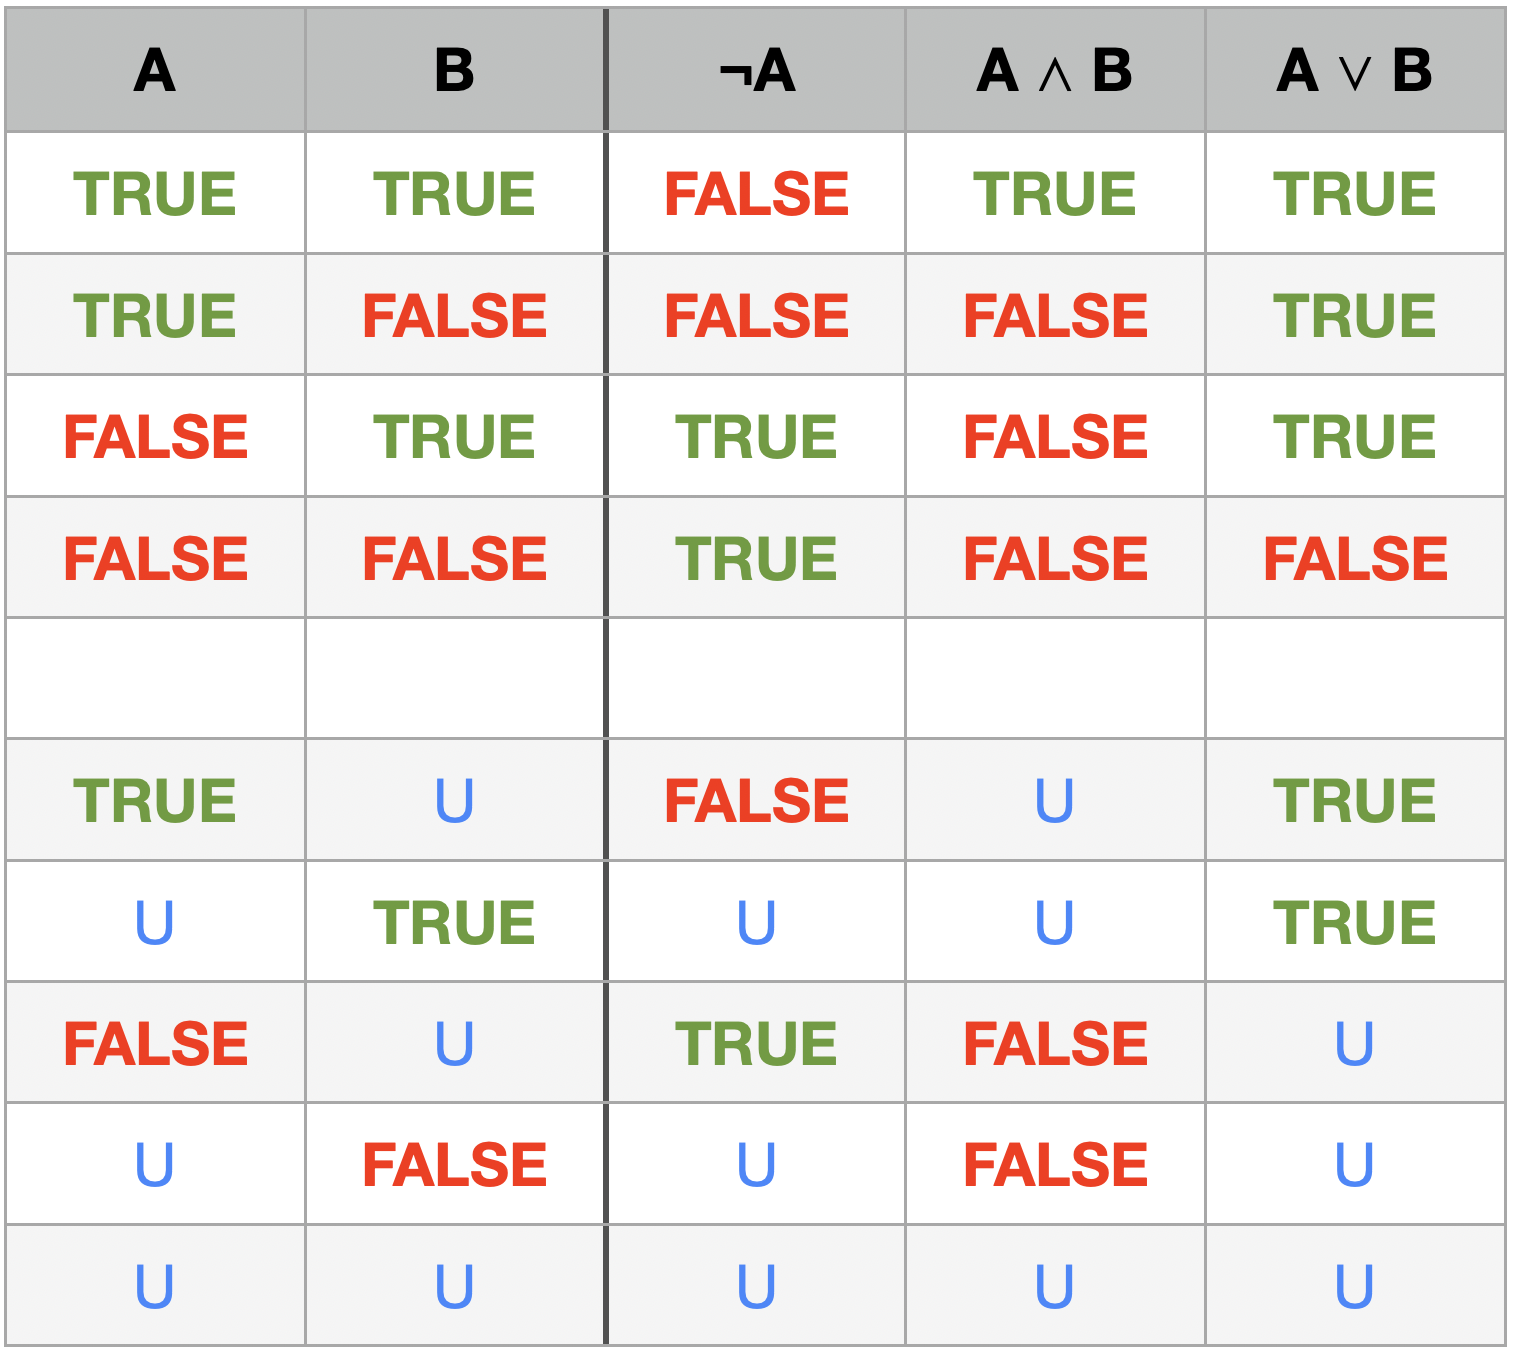}

In absence of null values, conditions in the WHERE never evaluate to the unknown value, and in this case three-valued logic (3VL) semantics coincides with classical two-valued logic (2VL) semantics. Indeed, \fosql queries without null values are equally expressive as classical \RA queries (see, e.g., \cite{ceri:gottlob:ieee-1985,VandenBussche:et:al:2009}).

Now, we are going to focus on the evaluation of the conditions in the \texttt{WHERE} clause. 

\begin{definition} [Simple comparison under 3VL semantics]
A simple comparison between two values evaluates under 3VL semantics to:
\begin{itemize}
	\item true if the two values do compare and each is different from NULL;  
	\item false if the two values don't compare and each is different from NULL;
	\item unknown if at least one value is NULL.
\end{itemize}
\end{definition} 

\begin{definition} [IS-NULL/IS-NOT-NULL simple comparison]
The IS-NULL unary simple comparison evaluates under 3VL semantics to:
\begin{itemize}
	\item true if the value is NULL;
	\item false if the value is not NULL.
\end{itemize}
The negation of the IS-NULL simple comparison is the IS-NOT-NULL unary simple comparison.
\end{definition} 

\begin{definition} [EXISTS/NOT-EXISTS atomic condition]
The EXISTS atomic condition evaluates under 3VL semantics to:
\begin{itemize}
	\item true if the query returns a non empty set of tuples;
	\item false otherwise.
\end{itemize}
The negation of the EXISTS atomic condition is the NOT-EXISTS atomic condition.
\end{definition} 

\begin{definition} [IN/NOT-IN atomic condition]
The IN atomic condition evaluates under 3VL semantics to:
\begin{itemize}
	\item true if the = simple comparison between the left expression and any element of the right expression set or of the result set of the query evaluates to true;
	\item false if the = simple comparison between the left expression and each element of the right expression set or of the result set of the query evaluates to false;
	\item unknown if the = simple comparison between the left expression and any element of the right expression set or of the result set of the query evaluates to unknown.
\end{itemize}
The negation of the IN atomic condition is the NOT-IN atomic condition.
\end{definition}

We observe that atomic conditions are closed under negation, so that an arbitrary level of negations in front of any atomic condition can be \textit{absorbed} in the usual way to obtain an atomic condition equivalent under 3VL semantics.

We now show that by normalising the condition in the WHERE clause, we can transform any \fosql query into an equivalent (under 3VL semantics) query where the condition does not contain any explicit negation.

\begin{lemma} [de Morgan with absorption]
de Morgan's laws are valid under 3VL semantics: it is always possible to normalise a boolean combination of atomic conditions under 3VL semantics to an equivalent (under 3VL semantics) negation normal form (NNF), where (possibly multiple levels of) negations appear only in front of atomic conditions. Negations can be absorbed, in order to obtain an equivalent (under 3VL semantics) absorbed negation normal form (ANNF) as a negation-free combination of conjunctions and disjunctions of atomic conditions.
\end{lemma}
\begin{proof}
Equivalence can be checked by using the 3VL truth tables with de Morgan's laws.\qed
\end{proof}

According to the \sql standard, the \texttt{SELECT} statement only considers rows for which the condition in the \texttt{WHERE} clause evaluates to true under 3VL semantics. If the condition is in absorbed negation normal form, we show that we can evaluate the condition under the classical 2VL semantics with the proviso of evaluating each atomic condition to false if it evaluates to unknown under 3VL semantics. 

\begin{definition} [Atomic conditions under classical 2VL semantics]
	An atomic condition under classical 2VL semantics evaluates to true if and only if it evaluates to true under 3VL semantics and it evaluates to false otherwise.
\end{definition}

\begin{lemma} [Equivalence of WHERE clause]
A boolean combination of atomic conditions evaluates to true under 3VL semantics
if and only if
the absorbed negation normal form of the boolean combination of atomic conditions under classical 2VL semantics evaluates to true.
\end{lemma}
\begin{proof}
Equivalence can be checked by using the 3VL truth tables with de Morgan's laws.\qed
\end{proof}

While the simple comparisons are simply implementable under classical 2VL semantics, and the 3VL semantics of EXISTS/NOT-EXISTS atomic conditions coincides with the classical 2VL semantics, the IN/NOT-IN atomic conditions are not directly implementable under classical 2VL semantics. Therefore, we report here a linear translation of the IN/NOT-IN atomic conditions under classical 2VL semantics into simple comparisons and the EXISTS/NOT-EXISTS atomic condition.

%\begin{lemma} [IN/NOT-IN atomic condition under classical 2VL semantics]
%A IN/NOT-IN atomic condition can always be translated into an equivalent condition under classical 2VL semantics as follows:

{\small
\begin{lstlisting}
e1 ... en IN (f1 ... fn) $\leadsto$
  e1 = f1 OR ... OR en = fn
\end{lstlisting}
\begin{lstlisting}
e1 ... en NOT IN (f1 ... fn) $\leadsto$
  e1 != f1 AND ... AND en != fn
\end{lstlisting}
\begin{lstlisting}
e1 ... en IN (q) $\leadsto$
  EXISTS (SELECT DISTINCT v.1 ... v.n FROM q AS v WHERE 
           e1 = v.1 AND ... AND en = v.n)
\end{lstlisting}
\begin{lstlisting}
e1 ... en NOT IN (q)) $\leadsto$
  NOT EXISTS (SELECT DISTINCT v.1 ... v.n FROM q AS v WHERE 
               ((e1 = v.1 OR e1 IS NULL) OR v.1 IS NULL) 
                 AND ... AND
               ((en = v.n OR en IS NULL) OR v.n IS NULL))
\end{lstlisting}}
%\end{lemma}

The main theorem can now be stated.

\begin{theorem} [Algebra counterpart of \fosql] 
A \fosql query, once the condition in the WHERE clause is transformed to an absorbed negation normal form, can be encoded into \nRA using the standard transformation for null-free \fosql in \RA (e.g., see \cite{ceri:gottlob:ieee-1985,VandenBussche:et:al:2009}), by considering the null value as any other value, and using the atomic conditions under classical 2VL semantics. The dual transformation is also possible using the standard dual transformation. Note that the basic \nRA considered in Figure~\ref{fig:nra} has only equality and inequality as atomic conditions.
\end{theorem}

\begin{corollary}  [\fosql and \nRA]
\fosql and \nRA are equally expressive.
\end{corollary}

%Let's consider now the semantics of the CHECK constraints. 
%
%According to the SQL standard, a check constraint CHECK(condition) is satisfied if and only if the condition evaluates to true or unknown. We can equivalently say, under 3VL semantics, that a check constraint CHECK(condition) is satisfied if and only if the negation of the condition does not evaluate to true. 
%%Indeed, CHECK(condition) defined on a table t is satisfied if and only if
%%NOT EXISTS ( SELECT * FROM t WHERE NOT ( condition ))
%%yields true.
%This is different from the 3VL semantics of the WHERE condition which is satisfied if and only if
%the condition evaluates to true. Under 3VL semantics, the WHERE condition is stronger than the CHECK condition. By mistakenly considering check constraints directly under classical 2VL semantics, the WHERE condition would be the same as the CHECK condition.
%
%In order to encode in \nRA a check constraint, we first transform its \emph{negated} condition to an absorbed negated normal form, and then we treat it as a \emph{denial} constraint with atomic conditions under classical 2VL semantics.
%
%
